# Supplementary material for: Vision-based Perimeter Defense via Multiview Pose Estimation
Source: arXiv:2209.12136 source file (2022-09-25)
Supplement: Supplementary file 1 [file 7.appendix.tex]

\section*{APPENDIX \label{sec:appendix}}

%%%%%%%%%%%%%%%%%  SUBSECTION  %%%%%%%%%%%%%%%%%%%%
\subsection{\blue{Optimal breaching point}}
\blue{
Given $\zd$, $\za$, we call $\textit{breaching point}$ as a point on the perimeter at which the intruder aims to reach the target, as shown $B$ in Fig.~\ref{fig:coord}. We call the azimuth angle that forms the breaching point as \textit{breaching angle}, denoted by $\theta$, and call the angle between $(\mf z_A - \mf z_B)$ and the tangent line at $B$ as \textit{approach angle}, denoted by $\beta$. }
\blue{
It is proved in \cite{lee2020perimeter} that given the current positions of defender $\mf z_D$ and intruder $\mf z_A$, there exists a unique breaching point such that the optimal strategy for both defender and intruder is to move towards it, known as \textit{optimal breaching point}. The breaching angle and approach angle corresponding to the optimal breaching point are known as \textit{optimal breaching angle}, denoted by $\theta^*$, and \textit{optimal approach angle}, denoted by $\beta^*$. As stated in \cite{lee2020perimeter}, we can form two governing equations:}
\begin{equation}
\beta^* =  \cos^{-1}\left(\nu\frac{\cos{\phi_D}\sin{\theta^*}}{\sqrt{1-\cos^2{\phi_D}\cos^2{\theta^*}}}\right)
\label{eq:beta}
\end{equation}
\blue{and}
\bql
\theta^* = \psi-\beta^*+\cos^{-1}\left(\frac{\cos\beta^*}{r}\right) \label{eq:theta},
\eql
\blue{with no closed-form solution for $\theta^*$ and $\beta^*$, but the solution can be computed by nonlinear equations solver.
}

%%%%%%%%%%%%%%%%%  SUBSECTION  %%%%%%%%%%%%%%%%%%%%
\subsection{\blue{Terminal time}}
\blue{In the hemisphere coordinate, the game ends at time $t_f$ with intruder's win if $r(t_f)\leq R$ and $|\psi(t_f)| + |\phi_D(t_f)|>0$,
whereas it ends with defender's win if $\phi_D(t_f)=\psi(t_f)=0$ and $r(t_f)>R$. 
We call $t_f$ as the \textit{terminal time}. }

%%%%%%%%%%%%%%%%%  SUBSECTION  %%%%%%%%%%%%%%%%%%%%
\subsection{Training curves in Section \ref{sec:training}}
In Fig. \ref{fig:training}, training curves show the train and validation loss for UV, Y, and total for the backbone as MobileNet\cite{howard2017mobilenets}, SqueezeNet\cite{iandola2016squeezenet}, MnasNet \cite{tan2019mnasnet}, and ShuffleNet \cite{zhang2018shufflenet}.
